# Supplementary material for: Robust Optimization as Data Augmentation for Large-scale Graphs
Source: arXiv:2010.09891 source file (2022-03-29)
Supplement: Supplementary file 1 [file appendix.tex]

\begin{table}[t]
\footnotesize
\caption{\texttt{ogbn-products}}
\centering
\begin{tabular}{lcccc}
\hline
 Backbone	 & Val Acc & $\alpha_l$ & $\alpha_u/\alpha_l$ & $M$  \\
\hline\hline
MLP         & 75.54\textcolor{gray}{\footnotesize{$\pm$0.14}}     &    -          &      -               &-     \\
+FLAG       &  76.88 \textcolor{gray}{\footnotesize{$\pm$0.14}}    &    2e-02           &      -               & 3 \\
\hline
GraphSAGE    & 91.70\textcolor{gray}{\footnotesize{$\pm$0.09}}  & -  & - & -   \\
+FLAG   & 92.05\textcolor{gray}{\footnotesize{$\pm$0.07}} &8e-03 & 2 & 3           \\
\hline
GAT     &   -     & - & - &-          \\
+FLAG   & 92.51\textcolor{gray}{\footnotesize{$\pm$0.06}}  & 5e-03 &2&3           \\
\hline
DeeperGCN   & 92.38\textcolor{gray}{\footnotesize{$\pm$0.09}}&-&-&-    \\
+FLAG    & 92.21\textcolor{gray}{\footnotesize{$\pm$0.37}}&5e-03&2&3          \\
\hline
	\end{tabular}
\end{table}

\begin{table}[t]
\footnotesize
\caption{\texttt{ogbn-proteins}}
\centering
\begin{tabular}{lcccc}
\hline
 Backbone & Val ROC-AUC & $\alpha_l$ & $\alpha_u/\alpha_l$ & $M$  \\
\hline\hline
GCN &  79.21\textcolor{gray}{\footnotesize{$\pm$0.18}} &-&-&-               \\
+FLAG &  78.93\textcolor{gray}{\footnotesize{$\pm$0.16}} &1e-03&1&3 \\
\hline
GraphSAGE   & 83.34\textcolor{gray}{\footnotesize{$\pm$0.13}} &-&-&-     \\
+FLAG & 82.84\textcolor{gray}{\footnotesize{$\pm$}0.17} &1e-03&1&3          \\
\hline
DeeperGCN  & 71.92\textcolor{gray}{\footnotesize{$\pm$0.16}}&-&-&-   \\
+FLAG & 91.32\textcolor{gray}{\footnotesize{$\pm$0.22}} &8e-03&1&3         \\
\hline
	\end{tabular}
\end{table}

\begin{table}[t]
\footnotesize
\caption{\texttt{ogbn-arxiv}}
\centering
\begin{tabular}{lcccc}
\hline
 Backbone & Val Acc & $\alpha_l$ & $\alpha_u/\alpha_l$ & $M$  \\
\hline\hline
MLP & 57.65\textcolor{gray}{\footnotesize{$\pm$0.17}} &-&-&-             \\
+FLAG & 58.17\textcolor{gray}{\footnotesize{$\pm$0.11}} &2e-03&-&3           \\
\hline
GCN & 73.00\textcolor{gray}{\footnotesize{$\pm$0.17}} &-&-&-             \\
+FLAG & 73.30\textcolor{gray}{\footnotesize{$\pm$0.10}}&1e-03&1&3    \\
\hline
GraphSAGE  & 72.77\textcolor{gray}{\footnotesize{$\pm$0.16}} &-&-&-     \\
+FLAG  & 73.49\textcolor{gray}{\footnotesize{$\pm$0.09}} &1e-03&1&3         \\
\hline
GAT   & 75.04\textcolor{gray}{\footnotesize{$\pm$0.06}} &-&-&-      \\
+FLAG    & 74.96\textcolor{gray}{\footnotesize{$\pm$0.10}} &1e-03&2&3         \\
\hline
DeeperGCN & 72.62\textcolor{gray}{\footnotesize{$\pm$0.14}} &-&-&- \\
+FLAG & 73.11\textcolor{gray}{\footnotesize{$\pm$0.09}} &8e-03&1&3      \\
\hline
	\end{tabular}
\end{table}

\begin{table}[t]
\footnotesize
\caption{\texttt{ogbn-mag}}
\centering
\begin{tabular}{lcccc}
\hline
 Backbone & Val Acc & $\alpha_l$ & $\alpha_u/\alpha_l$ & $M$  \\
\hline\hline
R-GCN & 47.61\textcolor{gray}{\footnotesize{$\pm$0.68}} &-&-&-  \\
+FLAG & 48.35\textcolor{gray}{\footnotesize{$\pm$0.36}}&1e-04&1&3             \\
\hline
	\end{tabular}
\end{table}

\begin{table}[t]
\footnotesize
\caption{\texttt{ogbg-molhiv}}
\centering
\begin{tabular}{lccc}
\hline
Backbone 	& Val ROC-AUC & $\alpha$ & $M$ \\
\hline\hline
GCN & 82.04\textcolor{gray}{\footnotesize{$\pm$1.41}} &-&- \\
+FLAG & 81.76\textcolor{gray}{\footnotesize{$\pm$0.87}} &1e-02 &3\\
\hline
GCN-Virtual & 83.84\textcolor{gray}{\footnotesize{$\pm$0.91}}&-&-\\
+FLAG & 83.83\textcolor{gray}{\footnotesize{$\pm$1.15}} & 1e-03 &3\\
\hline
GIN & 82.32\textcolor{gray}{\footnotesize{$\pm$0.90}} &-&-\\
+FLAG & 82.25\textcolor{gray}{\footnotesize{$\pm$1.55}} &5e-03 &3 \\
\hline
GIN-Virtual & 84.79\textcolor{gray}{\footnotesize{$\pm$0.68}} &-&-\\
+FLAG & 84.38\textcolor{gray}{\footnotesize{$\pm$1.28}} &1e-03 &3 \\
\hline
DeeperGCN & 84.27\textcolor{gray}{\footnotesize{$\pm$0.63}} &-&-\\
+FLAG & 84.25\textcolor{gray}{\footnotesize{$\pm$0.61}} & 1e-02 &3\\
\hline
\end{tabular}
\end{table}

\begin{table}[t]
\footnotesize
\caption{\texttt{ogbg-molpcba}}
\centering
\begin{tabular}{lccc}
\hline
Backbone  & Val AP & $\alpha$ & $M$ \\
\hline\hline
GCN  & 20.59\textcolor{gray}{\footnotesize{$\pm$0.33}} &-&-\\
+FLAG & 21.50\textcolor{gray}{\footnotesize{$\pm$0.22}} &8e-03&3\\
\hline
GCN-Virtual & 24.95	\textcolor{gray}{\footnotesize{$\pm$0.42}} &-&- \\
+FLAG & 25.56\textcolor{gray}{\footnotesize{$\pm$0.40}} & 8e-03&3 \\
\hline
GIN & 23.05\textcolor{gray}{\footnotesize{$\pm$0.27}} &-&-\\
+FLAG & 24.51\textcolor{gray}{\footnotesize{$\pm$0.42}} &8e-03&3 \\
\hline
GIN-Virtual & 27.98\textcolor{gray}{\footnotesize{$\pm$0.25}}&-&-\\
+FLAG & 29.12\textcolor{gray}{\footnotesize{$\pm$0.26}} &8e-03&3\\
\hline
DeeperGCN & 29.20\textcolor{gray}{\footnotesize{$\pm$0.25}}&-&-\\
+FLAG & 29.52\textcolor{gray}{\footnotesize{$\pm$0.29}} &8e-03&3\\
\hline
\end{tabular}
\end{table}

\begin{table}[t]
\footnotesize
\caption{\texttt{ogbg-ppa}}
\centering
\begin{tabular}{lccc}
\hline
Backbone & Val Acc & $\alpha$ & $M$ \\
\hline\hline
GCN & 64.97\textcolor{gray}{\footnotesize{$\pm$0.34}} &-&-\\
+FLAG & 64.98\textcolor{gray}{\footnotesize{$\pm$0.45}} & 2e-03 &3\\
\hline
GCN-Virtual & 65.11\textcolor{gray}{\footnotesize{$\pm$0.48}} &-&-\\
+FLAG & 66.38\textcolor{gray}{\footnotesize{$\pm$0.55}} &5e-03&3\\
\hline
GIN & 65.62\textcolor{gray}{\footnotesize{$\pm$1.07}}  &-&-\\ 
+FLAG & 64.65\textcolor{gray}{\footnotesize{$\pm$0.70}} & 8e-03&3\\
\hline
GIN-Virtual & 66.78\textcolor{gray}{\footnotesize{$\pm$1.05}} &-&- \\
+FLAG & 67.89\textcolor{gray}{\footnotesize{$\pm$0.79}} &5e-03&3\\
\hline
DeeperGCN & 73.13\textcolor{gray}{\footnotesize{$\pm$0.78}}  &-&-\\
+FLAG & 74.84\textcolor{gray}{\footnotesize{$\pm$0.52}} &8e-03 & 3\\
\hline
\end{tabular}
\end{table}

\begin{table}[t]
\footnotesize
\caption{\texttt{ogbg-code}}
\centering
\begin{tabular}{lccc}
\hline
Backbone & Val F1 & $\alpha$ & $M$ \\
\hline\hline
GCN & 29.73\textcolor{gray}{\footnotesize{$\pm$0.14}} &-&-\\
+FLAG & 30.16\textcolor{gray}{\footnotesize{$\pm$0.16}} & 8e-03 & 3\\
\hline
GCN-Virtual & 30.62\textcolor{gray}{\footnotesize{$\pm$0.07}} &-&-\\
+FLAG & 30.99\textcolor{gray}{\footnotesize{$\pm$0.16}} & 8e-03 &3\\
\hline
GIN & 29.81\textcolor{gray}{\footnotesize{$\pm$0.14}} &-&-\\
+FLAG & 30.44\textcolor{gray}{\footnotesize{$\pm$0.39}} & 8e-03 &3\\
\hline
GIN-Virtual & 30.20\textcolor{gray}{\footnotesize{$\pm$0.16}} &-&-\\
+FLAG & 30.92\textcolor{gray}{\footnotesize{$\pm$0.35}} & 8e-03 & 3\\
\hline
\end{tabular}
\end{table}

\begin{table}[h]
\footnotesize
\caption{\texttt{ogbl-ddi}}
\centering
\begin{tabular}{lccc}
\hline
Backbone & Val Hits@20 & $\alpha$ & $M$ \\
\hline\hline
GCN & 55.50\textcolor{gray}{\footnotesize{$\pm$2.08}} &-&-\\
+FLAG & 53.87\textcolor{gray}{\footnotesize{$\pm$1.48}} & 3e-03 & 3\\
\hline
GraphSAGE & 62.62 \textcolor{gray}{\footnotesize{$\pm$0.37}} &-&-\\
+FLAG & 69.74\textcolor{gray}{\footnotesize{$\pm$0.37}} & 3e-03 &3\\
\hline
\end{tabular}
\end{table}

\begin{table}[h]
\footnotesize
\caption{\texttt{ogbl-collab}}
\centering
\begin{tabular}{lccc}
\hline
Backbone & Val Hits@50 & $\alpha$ & $M$ \\
\hline\hline
GCN & 52.63\textcolor{gray}{\footnotesize{$\pm$1.15}} &-&-\\
+FLAG & 54.33\textcolor{gray}{\footnotesize{$\pm$0.86}} & 3e-03 & 3\\
\hline
GraphSAGE & 56.88\textcolor{gray}{\footnotesize{$\pm$0.77}} &-&-\\
+FLAG & 57.25\textcolor{gray}{\footnotesize{$\pm$0.40}} & 3e-03 &3\\
\hline
\end{tabular}
\end{table}
